# Supplementary material for: Scalable Reinforcement Post-Training Beyond Static Human Prompts: Evolving Alignment via Asymmetric Self-Play
Source: arXiv:2411.00062 source file (2025-04-09)
Supplement: Supplementary file 1 [file appendix.tex]

\newpage
\section{Summary Table for Preference Alignment Algorithms Used}\label{app:table}
Here, we unify preference alignment algorithms with the notion of \textcolor{SlateBlue4}{\textit{contrastive ratio}} defined as:
\begin{align}
    \emphslate{\dlog} :=\dpoinner. \nonumber
\end{align}

Most existing alignment objectives can be seen as to maximize the (regularized) contrastive ratio. 
% Detailed explanations on notations and insights can be found in Appendix~\ref{app:survey}.
% \notes{check the trpo paper.}
% \notes{TODO: add the Nash Equilibrium based ones for general preference modeling.}

% \subsection{Offline Direct Preference Alignment}

\begin{table}[H]
\centering
\resizebox{0.8\columnwidth}{!}{%
\begin{tabular}{@{}ll@{}}
\toprule
\multicolumn{2}{c}{With Reference Model}    \\ \midrule
DPO~\citep{dpo}  &  $\ell_{\beta}(\pi_{\vtheta}) = - \log \left[\sigma\left(\beta \cdot  \emphslate{\dlog} \right)\right]$                   \\

% IPO~\citep{ipo}  & $\ell_{\beta}(\pi_{\vtheta}) = \left(\emphslate{\dlog} \textcolor{Maroon}{- \frac{1}{2\beta}} \right)^{\textcolor{Maroon}{2}}$ \\ 
% SLiC~\citep{slic} & $\ell_{\beta}(\pi_{\vtheta}) = \textcolor{Maroon}{\max}\left(\textcolor{Maroon}{1 - \beta \cdot  \emphslate{\dlog} } , \textcolor{Maroon}{0} \right)$                    \\ 

% R-DPO~\citep{dpo-length}      &    $\ell_{\beta, \alpha}(\pi_{\vtheta}) = - \log \left[\sigma\left(\beta \cdot  \emphslate{\dlog} \textcolor{Maroon}{- \alpha \cdot \left( |\vtau_{+}| - |\vtau_{-}|\right)}\right)\right]$                 \\

% DPO-Positive~\citep{smaug}  & $\ell_{\beta, \alpha}(\pi_{\vtheta}) = - \log \left[\sigma\left(\beta \cdot  \emphslate{\dlog} \textcolor{Maroon}{- \alpha \cdot \max \left( 0, \log\frac{\pi_{\text{ref}} (\vtau_{+})}{\pi_{\vtheta}(\vtau_{+})}\right)}\right)\right]$  \vspace{+3pt}\\ 

SPPO~\citep{self-play-gu}  & $\ell_{\beta}(\pi_{\vtheta}) = (\beta \cdot \textcolor{SlateBlue4}{\log \frac{\pi_{\boldsymbol{\theta}}\left(\boldsymbol{\tau}_{+}\right)}{\pi_{\text {ref }}\left(\boldsymbol{\tau}_{+}\right)}} - \frac{1}{2})^2 + (\beta \cdot \textcolor{SlateBlue4}{\log \frac{\pi_{\boldsymbol{\theta}}\left(\boldsymbol{\tau}_{-}\right)}{\pi_{\text {ref }}\left(\boldsymbol{\tau}_{-}\right)}} + \frac{1}{2})^2$   \vspace{+3pt}\\ 

\midrule
\multicolumn{2}{c}{Without Reference Model} \\ \midrule
SimPO~\citep{simpo} &  $ \ell_{\beta, \alpha}(\pi_{\vtheta}) = -\log \left[\sigma \left( \beta \cdot \emphslate{\dlogsimpo} \textcolor{Maroon}{-\alpha} \right)\right] $                   \\
ORPO~\citep{orpo} &   $\ell_{\beta}^{\text{ORPO}}(\pi_{\vtheta}) = - \log \left[\sigma\left(\beta \cdot  \emphslate{\dlogodds} \right)\right]$\footnote{mark}               \\ \bottomrule
\end{tabular}%
}
\caption{Offline preference alignment algorithms.}
\label{tab:offline}
\end{table}
\footnotetext{Here, $\frac{\pi_{\vtheta}}{1 - \pi_{\vtheta}}$ can be denoted as $\text{odds}_{\vtheta}$, indicating how likely the model $\vtheta$ to generate the trajectory $\vtau$ than not generating it.}

\newpage
% ======================================================
\section{A Detailed Survey on Preference Alignment Algorithms}\label{app:survey}
% \notes{To provide a table here summarizing all the major players.}
% ======================================================

\subsection{Preliminaries}
\paragraph{Markov Decision Process (MDP).} Consider an episodic finite-horizon Markov Decision Process $\calM = (H, \calS, \calA, \sP, r, \rho)$, where $H$ is the horizon length, $\calS$ is the state space, $\calA$ is the action space, $\sP$ is the transition probability such that $\sP: \calS \times \calA \rightarrow \Delta(\calS)$, $r$ is the reward function such that $r: \mathcal{S} \times \mathcal{A} \rightarrow \mathbb{R}$, and $\rho$ is the initial state distribution where $\rho \in \Delta(\mathcal{S})$\footnote{$\Delta(\mathcal{S}) = \left\{ p \in \mathbb{R}^{|\mathcal{S}|} : \sum_{\rvs \in \mathcal{S}} p(\rvs) = 1, p(\rvs) \geq 0, \forall \rvs \in \mathcal{S} \right\}$, that is the set of distributions over $\calS$.}. A policy $\pi: \calS \rightarrow \Delta{(\calA)}$ induces a distribution over trajectories $\vtau$. The process can be denoted as:
\begin{align}
    (\rvs_1, r_1) \xrightarrow{\rva_1} (\rvs_2, r_2) \xrightarrow{\rva_2}  \ldots (\rvs_{H}, r_{H}) \xrightarrow{\rva_{H}} (\rvs_{H+1}, r_{H+1}). 
\end{align}
We define $r(\vtau)=\sum_{h=1}^H r\left(\rvs_h, \rva_h\right)$ and $r(\vtau) \in [0, R_{\text{max}}]$ almost surely for $R_{\text{max}} > 0$. We denote $\pi(\vtau)=\prod_{h=1}^H \pi\left(\rva_h \mid \rvs_h\right)$. 

% \notes{TODO: add the classical contextual bandit view, where each full response is considered as an arm to pull, within the regret minimization framework.}

\paragraph{Token-Level MDP view for language modeling.} We take interpretation below~\citep{r2q,xpo}:
\begin{table}[H]
\centering
\label{tab:lm-glossary}
\resizebox{0.99\columnwidth}{!}{%
\begin{tabular}{ll}
\textit{Initial state} ($\rvs_1$) & The prompt to the language model, sampled from distribution $\rho$. \\
\textit{Action} ($\rva_h$) & Each \emph{token} outputted by the language model. \\
\textit{Subsequent states} ($\rvs_h$) & The context (concatenation of the prompt with output tokens) so far: $\rvs_h = [\rvs_1, \rva_{1:h-1}]$. \\
& Note that the state transition is \emph{deterministic} due to the direct concatenation.\\
\textit{Policy} ($\pi(\rva_h \mid \rvs_h)$) & Mapping the current context to a distribution over tokens in the vocabulary $\calA$. \\
\textit{Trajectory / Response} ($\vtau$) & $\left(\rva_1, \rvs_1\right), \ldots, \left(\rva_H, \rvs_H\right)$. Note that $\rva_{1:H}$ represents the full response by LM. \\
 & Sometimes, we abuse the notation $\vtau$ to refer to $\rva_{1:H}$.
\end{tabular}%
}
\end{table}
\vspace{-5pt}

The goal is to use this preference data to train a policy that generates high-reward trajectories, that is to maximize:
\begin{align}
    J(\pi) 
    &= \sE_{\vtau \sim \pi(\vtau)} \left[ r(\vtau)\right] \\
    &= \sE_{\rva_h \sim \pi(\cdot \mid \rvs_h)} \left[ \sum_{h=1}^{H} r(\rvs_h, \rva_h)  \mid \rvs_0 \sim \rho(\rvs_0)\right] 
\end{align}

% \paragraph{Offline RLHF.} Given an offline labeled preference dataset, the RLHF objective is to maximize 

\paragraph{Offline RLHF.} Given an offline labeled preference dataset, the classical RLHF objective is to maximize the \emph{KL-regularized} expected cumulative rewards of the policy from the language model, where (i) the rewards often come from a human preference dataset $\calD_{\text{pref}}$, and (ii) the policy is regularized to be close to some reference policy $\pi_{\text{ref}}$. 

\begin{table}[!h]
\centering
\label{tab:rlhf-glossary}
\resizebox{0.99\columnwidth}{!}{%
\begin{tabular}{ll}
\textit{Reference Policy} ($\pi_{\text{ref}}$) & A policy typically obtained via supervised fine-tuning on a large corpus of data. \\
\textit{Preference Distribution} ($\sP_{\text{pref}}$) & A distribution over a binary preference for a response pair.\\
\textit{Preference Dataset} ($\mathcal{D}_{\text{pref}}$) & A set of labeled pairs of trajectories $(\vtau_{+}, \vtau_{-})$, indicating preferences. \\
 & Each pair is constructed by sampling $\vtau, \widetilde{\vtau} \sim \pi_{\text{ref}} \mid \rvs_1$ then annotating via $\vtau \succ \widetilde{\vtau} \mid \rvs_1$. \\
\textit{Bradley-Terry Model} & A probabilistic model for preferences, defined as $\mathbb{P}(\vtau \succ \widetilde{\vtau} \mid \rvs_1) = \frac{\exp (r(\vtau))}{\exp (r(\vtau)) + \exp (r(\widetilde{\vtau}))}$. \\
% \textit{KL-Regularized Reward Objective} ($J_\beta(\pi)$) & The objective function to maximize, defined as $J(\pi) - \beta \cdot \sum_{h=1}^H \mathbb{E}_\pi \left[D_{\mathrm{KL}} \left(\pi(\cdot \mid s_h) \| \pi_{\text{ref}}(\cdot \mid s_h)\right)\right]$. \\
\textit{Regularization Parameter} ($\beta$) & A parameter to balance reward maximization and closeness to the reference $\pi_{\text{ref}}$. \\
 & As $\beta$ gets smaller, the LM may generate more novel responses as opposed to reference.
\end{tabular}%
}
\end{table}

The RLHF objective is then to maximize:
\begin{align}
    J_{\beta}(\pi) &= J(\pi) - \beta \cdot \mathbb{D}_{\mathrm{KL}}\left[\pi(\vtau) \| \pi_{\mathrm{ref}}(\vtau)\right] \\
    &= \sE_{\vtau \sim \pi(\vtau)} \left[ r(\vtau) - \beta \cdot \log \frac{\pi(\vtau)}{\pi_{\text{ref}}(\vtau)}\right] \label{eq:rlhf-2} \\
    &= \sE_{\rva_h \sim \pi(\cdot \mid \rvs_h)} \left[ \sum_{h=1}^{H} \left( r(\rvs_h, \rva_h) -\beta \log \frac{\pi\left(\rva_h \mid \rvs_h\right)}{\pi_{\mathrm{ref}}\left(\rva_h \mid \rvs_h\right)} \right)  \mid \rvs_0 \sim \rho(\rvs_0)\right]. 
    %= \underset{\rva_h \sim \pi(\cdot \mid \rvs_h)}{\sE}
\end{align}

For some small $\epsilon > 0$, the goal is to compute an $\epsilon$-optimal policy $\hat{\pi}$ such that: 
\begin{align}
    \max _\pi J_\beta(\pi)-J_\beta(\widehat{\pi}) \leq \varepsilon.
\end{align}

The DPO objective~\citep{dpo} is to minimize:
\begin{align}
    \calL_{\beta}^{\text{DPO}}(\pi) = \sum_{\left(\vtau_{+}, \vtau_{-}\right) \in \mathcal{D}_{\text {pref}}} - \log \left[\sigma\left(\beta \cdot  \log \frac{\pi\left(\vtau_{+}\right)}{\pi_{\text{ref}}\left(\vtau_{+}\right)}-\beta \cdot \log \frac{\pi\left(\vtau_{-}\right)}{\pi_{\mathrm{ref}}\left(\vtau_{-}\right)}\right)\right],
\end{align}
where $\sigma(\cdot)$ is the sigmoid function. Without loss of generality, we denote $J_{\beta}^{\text{DPO}}(\pi_{\vtheta}) := - \calL_{\beta}^{\text{DPO}}(\pi_{\vtheta})$, with the loss function:
\begin{align}
\ell_{\beta}^{\text{DPO}}(\pi_{\vtheta}) = - \log \left[\sigma\left(\beta \cdot  \emphslate{\dlog} \right)\right],
\end{align}
where we define the \textcolor{SlateBlue4}{\emph{contrastive ratio}} as:
\begin{align}
    \emphslate{\dlog} :=\dpoinner. \label{eq:contrastive-ratio}
\end{align}

We introduce more formulations below. A major direction is to add different offset terms to modulate the difference between (i) $\pi_{\vtheta}(\vtau_-)$ and $\pi_{\vtheta}(\vtau_+)$, and/or (ii) $\pi_{\vtheta}(\cdot)$ and $\pi_{\text{ref}}(\cdot)$.

\begin{itemize}
    \item \textbf{DPO}~\citep{dpo}: the loss pushes $\textcolor{SlateBlue4}{\beta \cdot} \dlog \textcolor{SlateBlue4}{\rightarrow \infty}$, \ie being as large as possible \emph{unboundly}:
    \begin{align}
    \ell_{\beta}^{\text{DPO}}(\pi_{\vtheta}) = - \log \left[\sigma\left(\beta \cdot  \emphslate{\dlog} \right)\right],
    \end{align}

    \item \textbf{R-DPO}~\citep{dpo-length}: the loss pushes $\textcolor{SlateBlue4}{\beta \cdot} \dlog \textcolor{SlateBlue4}{\rightarrow \infty}$ while encouraging a relatively smaller response length for $\vtau_{+}$:
    \begin{align}
    \ell_{\beta}^{\text{R-DPO}}(\pi_{\vtheta}) = - \log \left[\sigma\left(\beta \cdot  \emphslate{\dlog} \textcolor{Maroon}{- \alpha \cdot \left( |\vtau_{+}| - |\vtau_{-}|\right)}\right)\right].
    \end{align}
    
    \item \textbf{IPO}~\citep{ipo}: the loss pushes  $\textcolor{SlateBlue4}{\beta \cdot} \dlog \textcolor{SlateBlue4}{\rightarrow 1/2}$, \ie being as close to a constant as possible:
    \begin{align}
        \ell_{\beta}^{\text{IPO}}(\pi_{\vtheta}) = \left(\emphslate{\dlog} \textcolor{Maroon}{- \frac{1}{2\beta}} \right)^{\textcolor{Maroon}{2}}.
    \end{align}

        \item \textbf{SLiC}~\citep{slic}: the loss pushes $\textcolor{SlateBlue4}{\beta \cdot} \dlog \textcolor{SlateBlue4}{\geq 1}$, and halts \emph{whenever the threshold is reached}:
    \begin{align}
        \ell_{\beta}^{\text{SLiC}}(\pi_{\vtheta}) = \textcolor{Maroon}{\max}\left(\textcolor{Maroon}{1 - \beta \cdot  \emphslate{\dlog} } , \textcolor{Maroon}{0} \right).
    \end{align}

    \item \textbf{DPO-Positive}~\citep{smaug}: The primary objective is the same as DPO, while adding an additional penalty term, which discourage the current policy from assigning a lower probability to $\vtau_+$, compared to the reference policy. A higher $\alpha$ increases the penalty, making the policy more conservative w.r.t. the reference policy.
    \begin{align}
    \ell_{\beta}^{\text{DPOP}}(\pi_{\vtheta}) = - \log \left[\sigma\left(\beta \cdot  \emphslate{\dlog} \textcolor{Maroon}{- \alpha \cdot \max \left( 0, \log\frac{\pi_{\text{ref}} (\vtau_{+})}{\pi_{\vtheta}(\vtau_{+})}\right)}\right)\right].
    \end{align}
\end{itemize}

Additionally, there are reference-free variants:
\begin{itemize}

    \item \textbf{SimPO}~\citep{simpo}: the loss pushes  $\textcolor{SlateBlue4}{\beta \cdot} \dlogsimpo \textcolor{SlateBlue4}{\rightarrow \infty}$, for the \emph{length-normalized, reference-free} contrastive ratio to be as large as possible \emph{unboundly}, modulated by \(\gamma\). A higher reward margin $\gamma$ means the contrastive ratio needs to be larger to achieve the same reduction in loss, essentially requiring the log-likelihood of the preferred examples to be higher relative to that of the un-preferred ones.
    \begin{align}
         \ell_{\beta}^{\text{SimPO}}(\pi_{\vtheta}) &= -\log \left[\sigma \left( \beta \cdot \emphslate{\dlogsimpo} \textcolor{Maroon}{-\gamma} \right)\right] \\
         &=-\log \left[\sigma \left( \beta \cdot \left(  \log \pi_\theta\left(\vtau _{+} \right) ^{\frac{1}{|\vtau _{+}|}} - \log \pi_\theta\left( \vtau_ {-}\right) ^{\frac{1}{|\vtau_{-}|}} \right) -\gamma \right)\right].
    \end{align}
    % \begin{align}
    %     &-\log \left[\sigma \left( \beta \cdot \left( \frac{1}{\left|y_w\right|} \log \pi_\theta\left(y_w \mid x\right)-\frac{1}{\left|y_l\right|} \log \pi_\theta\left(y_l \mid x\right) \right) -\gamma \right)\right] \\
    %     &=-\log \left[\sigma \left( \beta \cdot \left(  \log \pi_\theta\left(\vtau _{+} \right) ^{\frac{1}{|\vtau _{+}|}} - \log \pi_\theta\left( \vtau_ {-}\right) ^{\frac{1}{|\vtau_{-}|}} \right) -\gamma \right)\right] \\
    %     &= -\log \left[\sigma \left( \beta \cdot \Delta_{\log}\left(\pi_{\vtheta}^{\frac{1}{|\vtau|}}, 1 \right) -\gamma \right)\right]
    % \end{align}

    \item \textbf{ORPO}~\citep{orpo}: the loss will push up the odds (\ie $\pi_{\vtheta} / (1 - \pi_{\vtheta})$) on the preferred trajectory, while pushing down the odds on the less preferred trajectory.
    \begin{align}
    \ell_{\beta}^{\text{ORPO}}(\pi_{\vtheta}) = - \log \left[\sigma\left(\beta \cdot  \emphslate{\dlogodds} \right)\right].
    \end{align}

\end{itemize}

\paragraph{Online RLHF.} Instead of using a static $\calD_{\text{ref}}$, online RLHF method grows and sample from a different $\calD_{\text{pref}}^{(t)}$ for each time step or episode $t$. The process can be summarized as (i) response sampling from the online policy, (ii) preference labeling by human or AI annotators, (iii) dataset updating with the new preference pair, and (iv) policy update with some loss function. 

Essentially, this approach gains new information from the environment by the online sampling and preference labeling process. Assuming a perfect oracle for the preference labeling, the challenge will more come from the  exploration v. exploitation dilemma.

\begin{itemize}
    \item \textbf{OAIF}~\citep{dpo-ai-feedback}:
    \begin{itemize}
        \item \textbf{Response sampling}: sample a prompt from $\calD_{\text{pref}}$ then sample a tuple of responses from the \emph{online policy}:
        \begin{align}
            \vtau^{(t)} \sim \pi_{\vtheta}^{(t)}, \ \widetilde{\vtau}^{(t)} \sim \pi_{\vtheta}^{(t)}. \label{eq:online-response-sampling}
        \end{align}
        
        \item \textbf{Preference labeling}: sample the binary preference $y^{(t)} \sim \sP_{\text{pref}}\left(\vtau^{(t)} \succ \widetilde{\vtau}^{(t)}_{\text{ref}}\right)$, then apply it on the tuple to obtain:
        \begin{align}
            \left(\vtau_{+}^{(t)}, \vtau_{-}^{(t)}\right). \label{eq:online-pref-label}
        \end{align}
        
        \item \textbf{Dataset updating}: the original paper assumes batch size being 1, thus $\calD_{\text{pref}^{(t)}} = \left(\vtau_{+}^{(t)}, \vtau_{-}^{(t)}\right)$.

        \item \textbf{Policy updating}: use standard loss functions, albeit the optimization is taken over the online preference:
        \begin{align}
        \pi^{(t+1)}_{\vtheta} \leftarrow \underset{\pi \in \Pi}{\operatorname{argmin}}\left\{ \sum_{ \textcolor{Maroon}{\left(\vtau_{+}, \vtau_{-}\right) \in \mathcal{D}_{\text {pref}}^{(t)}} } \textcolor{black}{\ell_{\beta}^{\text{\{DPO, IPO, SLiC\}}}(\pi_{\vtheta})}\right\}   
        \end{align}
    \end{itemize}

    % \item \textbf{DNO}~\citep{dno}: The idea is that human preference may be \emph{intransitive}. The paper proposes to optimize such \emph{general preference} by finding the Nash equilibrium of the two-player zero-sum game by the min-max winner:
    % \begin{align}
    %     \operatorname{MW}(\sP) &:=\underset{\pi \in \Pi}{\operatorname{argmax}} \ \underset{\pi^{\prime} \in \Pi}{\operatorname{argmin}} \ \sP \left(\pi \succ \pi^{\prime}\right) \\
    %     &=\left(\underset{\pi \in \Pi}{\operatorname{argmax}} \min _{\pi^{\prime} \in \Pi} \sP\left(\pi \succ \pi^{\prime}\right) \ , \ \underset{\pi^{\prime} \in \Pi}{\operatorname{argmin}} \  \underset{\pi \in \Pi}{\max} \ \sP \left(\pi \succ \pi^{\prime}\right)\right)
    % \end{align}
    % \begin{itemize}
    %     \item \textbf{Response sampling}: for each prompt $i$ from $\calD_{\text{pref}}$, sample a tuple of responses from the \emph{online policy}:
    %     \begin{align}
    %         \vtau^{(t)}_i \sim \pi_{\vtheta}^{(t)}, \ \widetilde{\vtau}^{(t)}_i \sim \pi_{\vtheta}^{(t)}. 
    %     \end{align}
        
    %     \item \textbf{Preference labeling}:
        
    %     \item \textbf{Dataset updating}:
        
    %     \item \textbf{Policy updating}:
    % \end{itemize}

    % \item \textbf{Iterative RPO}~\citep{iterative-rpo}:
    
    % \item \textbf{Iterative DPO}~\citep{dpo-iterative}:
    % \begin{itemize}
    %     \item \textbf{Response sampling}:
        
    %     \item \textbf{Preference labeling}:
        
    %     \item \textbf{Dataset updating}:
        
    %     \item \textbf{Policy updating}:
    % \end{itemize}

    \item \textbf{SELM}~\citep{selm}:
    \begin{itemize}
        \item \textbf{Response sampling}: for {each prompt} $i$ in $\calD_{\text{pref}}$, generate \emph{a new response} $\vtau^{(t)}_i$.
        
        \item \textbf{Preference labeling}: for {each prompt} $i$ in $\calD_{\text{pref}}$, re-rank $\left(\vtau^{(t)}_i, \vtau_{i, +}^{(t-1)}, \vtau_{i, -}^{(t-1)} \right)$, then construct a new preference pair containing the best and the worst response to obtain $\left(\vtau_{+}^{(t)}, \vtau_{-}^{(t)}\right)$.
        
        \item \textbf{Dataset updating}: for {each prompt} $i$ in $\calD_{\text{pref}}$, update the response pair such that:
        \begin{align}
            \mathcal{D}_{\text {pref}}^{(t)} \gets \left\{\left(\vtau_{i,+}^{(t)}, \vtau_{i,-}^{(t)}\right)\right\}_{i=1}^{|\calD_{\text{pref}}|}. 
        \end{align}
        
        \item \textbf{Policy updating}: over $\mathcal{D}_{\text {pref }}^{(t)}$, calculate policy $\pi^{(t+1)}_{\vtheta}$ with \textcolor{RoyalBlue2}{optimism in the face of uncertainty}:
        \begin{align}
        \pi^{(t+1)}_{\vtheta} \leftarrow \underset{\pi \in \Pi}{\operatorname{argmin}}\left\{\sum_{ \textcolor{Maroon}{\left(\vtau_{+}, \vtau_{-}\right) \in \mathcal{D}_{\text {pref}}^{(t)}} } \textcolor{black}{\ell_{\beta}^{\text{DPO}}(\pi_{\vtheta})} \ + \emphblue{\textcolor{RoyalBlue2}{\ \alpha \cdot \sum_{i=1}^{|\calD_{\text{pref}}|} \log \pi_{\vtheta}\left({\vtau}^{(t)}_{i}\right)}} \right\}   
        \end{align}
        
    \end{itemize}

\end{itemize}
